# Supplementary material for: Improving Autoregressive Visual Generation with Cluster-Oriented Token Prediction
Source: arXiv:2501.00880 source file (2025-03-15)
Supplement: Supplementary file 1 [file X_suppl.tex]

\setcounter{equation}{0}
\setcounter{table}{0}
\setcounter{figure}{0}
\appendix

\section{Overview}
\label{sec:rationale}
The supplementary material is composed of:
\begin{itemize}

\item Implementation details (Sec.~\ref{sec:implementation details});

\item  More Analysis on our model (Sec.~\ref{sec:more analysis on our model});

\item More ablation studies (Sec.~\ref{sec: more ablation studies});

\item More visualized results (Sec.~\ref{sec: more visualized results});

\end{itemize}

\section{Implementation Details}
\label{sec:implementation details}

{\bf Metrics.}

{\bf Experiment settings.}

{\bf }

\section{More Analysis on Our Model}
\label{sec:more analysis on our model}

\section{More Ablation Studies}
\label{sec: more ablation studies}

\section{More Visulized Results}
\label{sec: more visualized results}
